# Supplementary material for: Rethinking Offensive Text Detection as a Multi-Hop Reasoning Problem
Source: arXiv:2204.10521 source file (2022-04-22)
Supplement: Supplementary file 1 [file appendix_H.tex]

\section{Knowledge Coverage Experiment}
\label{sec:appendixH}

Table~\ref{tab:prompt} shows the prompt used in the knowledge coverage experiment. In order to make sure that the models have access to the knowledge, we apply a 2-step conversational prompt. In step 1, the models are asked if they know the knowledge or not. In step 2, the model will have to give an reason to explain the knowledge. Based on the explanations we should be able verify the accessibility to the knowledge.

Figure~\ref{fig:knowledge_instruction} shows the instruction for annotators and Figure~\ref{fig:knowledge_ui} shows the interface used in the task. The annotators are asked to select if the generated explanations are able to explain the given knowledge. Given that the generated text may contain offensive contents, we have made specific clarification that the workers are able to report the examples that contain offensive contents and have the right to immediately stop the task.

We have filtered out all knowledge examples that are related to protected classes such as gender, race, etc. For each example of knowledge, we assign 5 annotators to vote for the final answers with the Krippendorff's $\alpha=0.724$. Given that removing protected classes related examples may create more biases on our evaluation, we have asked an expert to finish the evaluation task under the same condition however without protected classes removed. Table~\ref{tab:knowledge_coverage_expert} shows the evaluation results given by the expert.

\begin{figure*}
    \centering
    \includegraphics[width = \textwidth]{figure/knowledge_coverage_crowdsourcing.png}
    \caption{The instruction for annotators used in the knowledge coverage experiment.}
    \label{fig:knowledge_instruction}
\end{figure*}

\begin{figure*}
    \centering
    \includegraphics[width = \textwidth]{figure/knowledge_coverage_crowdsourcing_2.png}
    \caption{The interface used in the knowledge coverage experiment.}
    \label{fig:knowledge_ui}
\end{figure*}

Table~\ref{tab:knowledge_coverage} shows the knowledge coverage rate by different GPT models. The trend of improvement on knowledge coverage implies that with more training data and better engineering, pre-trained language models are able to gain more knowledge significantly. In our experiment, GPT-3 is able to cover $>70\%$ of the knowledge used in our dataset.

\begin{table*}[]
    \centering
    \begin{tabular}{l}
    \toprule
    Prompt: \\
    \midrule
    Q: Do you know that <knowledge>?  \\
    A: Yes.  \\
    Q: Why? \\
    A: \\ \hline
    Examples: \\ \hline
    Q: Do you know that junk food are unhealthy? \\
    A: Yes. \\
    Q: Why? \\
    A: Because junk food is high in calories and can cause obesity. \\
    \hline
    Q: Do you know that people hate disasters? \\
    A: Yes. \\
    Q: Why? \\
    A: Because they think that they are going to die. \\
    \bottomrule
    \end{tabular}
    \caption{The prompt used in knowledge accessibility experiment and some example answers by GPT-3.}
    \label{tab:prompt}
\end{table*}

\input{tables/knowledge_converage}
